# Supplementary material for: PeRFception: Perception using Radiance Fields
Source: arXiv:2208.11537 source file (2022-08-24)
Supplement: Supplementary file 2 [file mesh_reconstruction_quality.tex]

\begin{table}[!tb]
    \caption{Comparison of reconstruction quality of Co3D and \our Co3D. PSNR of rendered images is used as a proxy to assess the reconstruction quality. Object masks are applied to each image since the reconstructed point clouds of Co3D dataset do not include backgrounds}
    \centering
    \begin{tabular}{ccccc}
        \toprule
        Dataset & PSNR($\uparrow$) & \%(PSNR $>$ 15) & \%(PSNR $>$ 20) & \%(PSNR $>$ 25)\\
        \midrule
        Co3D & 18.49 & 84.83 & 34.48 & 2.83 \\
        \midrule
        \rowcolor{yellow!40}
        \our Co3D &\textbf{ 27.31} & \textbf{98.85} & \textbf{94.14} & \textbf{75.35} \\
        \bottomrule
    \end{tabular}
    \label{tab:recon_qual}
\end{table}

\begin{comment}
\begin{table}[!tb]
    \caption{Comparison of reconstruction quality of Co3D and \our Co3D. PSNR of rendered images is used as a proxy to assess the reconstruction quality. Object masks are applied to each image since the reconstructed point clouds of Co3D dataset do not include backgrounds}
    \centering
    \begin{tabular}{c|c|c|c|c}
        Dataset & PSNR($\uparrow$) & \%(PSNR $>$ 15) & \%(PSNR $>$ 20) & \%(PSNR $>$ 25)\\
        \hline
        Co3D & 18.59 & 85.19 & 34.99 & 2.90 \\
        \hline
        \rowcolor{yellow!40}
        \our Co3D &\textbf{ 27.31} & \textbf{98.85} & \textbf{94.14} & \textbf{75.35} \\
    \end{tabular}
    \label{tab:recon_qual}
\end{table}
\end{comment}
