# Supplementary material for: PeRFception: Perception using Radiance Fields
Source: arXiv:2208.11537 source file (2022-08-24)
Supplement: Supplementary file 3 [file ethical_concern.tex]

\revision{
\subsection{Ethical Implications}
Our dataset is capable of generating unseen views from multi-view images. Thus, realistic fake videos whose camera trajectories are different from the original video can be generated from our dataset. 
}
