# Supplementary material for: PeRFception: Perception using Radiance Fields
Source: arXiv:2208.11537 source file (2022-08-24)
Supplement: Supplementary file 4 [file rendering_scores.tex]

\subsection{Class-wise Rendering Quality}

We provide class-wise PSNR, SSIM, and LPIPS scores of \our CO3D dataset in Table~\ref{tab:supp_classwise}.
\input{assets/tables/supp/3_classwise}
